# Supplementary material for: Learning from Matured Dumb Teacher for Fine Generalization
Source: arXiv:2108.05776 source file (2021-08-17)
Supplement: Supplementary file 2 [file 3d_dt_cifar100_table.tex]

\begin{table}[h]
\centering
\begin{tabular}{l|llllllll}
\diagbox[]{$\alpha$}{$p_t$} 
& 0.5    & 0.6    & 0.7    & 0.8    & 0.9    & 0.99   & 0.999  & 0.9999 \\
\hline
0.001 & 76.09 & 76.42 & 76.12 & 75.89 & 76.56 & 74.93 & 76.25 & 75.54  \\
0.005 & 76.60 & 75.92 & 76.18 & 76.40 & 76.26 & 74.72 & 76.20 & 76.17  \\
0.01  & 76.46 & 76.64 & 76.46 & 76.49 & 76.05 & 74.93 & 76.87 & 76.98  \\
0.05  & 76.40 & 76.20 & 76.36 & 75.89 & 75.73 & 74.98 & 78.01 & \textbf{78.21}  \\
0.1   & 76.12 & 76.24 & 76.30 & 76.27 & 76.37 & 74.26 & 77.91 & 77.66  \\
0.15  & 76.37 & 76.44 & 75.89 & 76.29 & 75.22 & 74.00 & 77.95 & 78.03  \\
0.2   & 75.91 & 76.34 & 76.41 & 76.26 & 75.66 & 73.40 & 78.02 & 77.79  \\
0.3   & 76.26 & 76.15 & 76.29 & 76.43 & 75.51 & 73.11 & 78.20 & 78.03  \\
0.4   & 76.66 & 76.15 & 76.36 & 76.07 & 75.73 & 70.40 & 77.32 & 77.91  \\
0.5   & 76.30 & 76.85 & 76.55 & 76.20 & 74.97 & 67.45 & 77.46 & 77.73 
\end{tabular}
\caption{Accuracy values of CIFAR100 in Fig.~7, where $p_t$ is the dropout probability of a teacher, and $\alpha$ is the teacher rate in Equation~5.}
\end{table}
