# Supplementary material for: Learning from Matured Dumb Teacher for Fine Generalization
Source: arXiv:2108.05776 source file (2021-08-17)
Supplement: Supplementary file 3 [file 3d_dt_cifar10_table.tex]

\begin{table}[h]
\centering
\begin{tabular}{l|llllllll}
\diagbox[]{$\alpha$}{$p_t$} 
& 0.5    & 0.6    & 0.7    & 0.8    & 0.9    & 0.99   & 0.999  & 0.9999 \\
\hline
0.001 & 93.75 & 93.99 & 93.97 & 94.20 & 93.99 & 93.83 & 94.07 & 94.00  \\
0.005 & 93.83 & 94.09 & 93.98 & 94.05 & 93.91 & 94.00 & \textbf{94.56} & 94.36  \\
0.01  & 94.17 & 94.05 & 93.93 & 93.99 & 93.85 & 94.15 & 94.51 & 94.33  \\
0.05  & 93.94 & 94.12 & 93.98 & 94.00 & 94.13 & 94.22 & 94.36 & 94.32  \\
0.1   & 94.08 & 94.15 & 94.30 & 94.02 & 93.98 & 94.03 & 94.52 & 94.36  \\
0.15  & 94.29 & 93.93 & 93.88 & 94.30 & 93.74 & 93.80 & 94.26 & 94.34  \\
0.2   & 94.07 & 93.95 & 94.22 & 94.34 & 93.91 & 93.87 & 94.29 & 94.26  \\
0.3   & 94.14 & 93.94 & 94.24 & 94.12 & 93.68 & 93.24 & 94.26 & 94.31  \\
0.4   & 94.26 & 94.13 & 94.35 & 93.93 & 93.17 & 92.35 & 94.19 & 94.26  \\
0.5   & 94.22 & 93.93 & 94.10 & 94.12 & 92.87 & 90.51 & 94.17 & 94.23 
\end{tabular}
\caption{Accuracy values of CIFAR10 in Fig.~7, where $p_t$ is the dropout probability of a teacher, and $\alpha$ is the teacher rate in Equation~5.}
\end{table}
