# Supplementary material for: Learning from Matured Dumb Teacher for Fine Generalization
Source: arXiv:2108.05776 source file (2021-08-17)
Supplement: Supplementary file 4 [file 3d_dt_mnist_table.tex]

\begin{table*}[h]
\centering
\begin{tabular}{l|llllllll}
\diagbox[]{$\alpha$}{$p_t$} 
& 0.6    & 0.7    & 0.8    & 0.9    & 0.95   & 0.99   & 0.999  & 0.9999 \\
\hline
0.001 & 98.24 & 98.31 & 98.26 & 98.30 & 98.26 & 98.40 & 98.35 & 98.21  \\
0.005 & 98.25 & 98.25 & 98.25 & 98.19 & 98.20 & 98.47 & 98.33 & 98.16  \\
0.01  & 98.26 & 98.26 & 98.25 & 98.20 & 98.19 & 98.54 & 98.33 & 98.15  \\
0.05  & 98.29 & 98.24 & 98.27 & 98.15 & 98.09 & 98.52 & 98.15 & 97.95  \\
0.1   & 98.24 & 98.24 & 98.25 & 98.12 & 97.99 & 98.55 & 98.00 & 97.51  \\
0.2   & 98.23 & 98.24 & 98.28 & 98.05 & 97.85 & 98.53 & 97.42 & 96.28  \\
0.3   & 98.28 & 98.22 & 98.27 & 97.95 & 97.71 & \textbf{98.63} & 96.28 & 93.57  \\
0.4   & 98.23 & 98.22 & 98.26 & 97.94 & 97.54 & 98.59 & 93.54 & 87.11  \\
0.5   & 98.24 & 98.23 & 98.26 & 97.92 & 97.28 & 98.57 & 89.11 & 79.14  \\

\end{tabular}
\caption{Accuracy values of MNIST in Fig.~7, where $p_t$ is the dropout probability of a teacher, and $\alpha$ is the teacher rate in Equation~5.}
\end{table*}
